# Supplementary material for: Multi-scale Dynamic and Hierarchical Relationship Modeling for Facial Action Units Recognition
Source: arXiv:2404.06443 source file (2024-04-09)
Supplement: Supplementary file 1 [file X_suppl.tex]

\clearpage
\setcounter{page}{1}

\maketitle
% \maketitlesupplementary
\footnotetext{Corresponding author}

\section{Details of the employed TCN and SC}

\noindent We provide the details of the temporal convolution Network (TCN) and the similarity calculating (SC) strategy employed in the proposed MDHR model. While the MFD module computes short-term facial dynamics between neighboring frames, long-term facial dynamics ($T$ frames) are failed to be considered, which may provide additional cues for AU recognition. Consequently, we incorporate channel-wise temporal convolution network into our MDHR framework. For the $n_{th}$ AU, the $n_{th}$ graph nodes corresponding to the $T$ input frames (produced by the GAT layer) are considered as an AU sequence  $\hat{V}_n = \{ \hat{v}_{n}^{1}, \cdots, \hat{v}_{n}^{t}, \cdots, \hat{v}_{n}^{T} \} \in \mathbb{R}^{T \times b}$. As a result, $N$ AU sequences are obtained, where each is fed to a TCN to model long-term facial dynamics. This way, the AU node sequence $\hat{V}_n$ is updated as:
\begin{equation}
\Bar{V}_n = \text{Conv1D}_n(\hat{V}_n)
\end{equation}
where the $\Bar{V}_n = \{ \Bar{v}_{n}^{1}, \cdots, \bar{v}_{n}^{t}, \cdots, \bar{v}_{n}^{T} \} \in \mathbb{R}^{T \times b}$ denotes the obtained long-term facial dynamic-aware representations of the $n_\text{th}$ AU for the input $T$ frames; and the kernel size of the temporal convolution operation is $5 \times1 $. Then, the similarity calculating (SC) strategy is employed to predict the probability of each AU's occurrence. For the $n_{th}$ AU, a trainable vector $s_n$ that has the same dimension as $\bar{v}_{n}^{t}$ is shared across all $T$ frames, based on which the $n_{th}$ AU prediction of the $t_{th}$ frame is made as:
\begin{equation}
 p_{n}^{t} = \frac{\sigma(\bar{v}_{n}^{t})^T \sigma(s_n)}{|| \sigma(\bar{v}_{n}^{t}) ||_2 || \sigma(s_n)||_2}   
\end{equation}
where $\sigma$ is an activation function.

\section{Target AUs of each facial region}

Table \ref{tab:rules} displays the target AUs located in each facial region defined by our approach, which are labelled by either BP4D or DISFA datasets.

\begin{table}[h!]
    \centering
    \begin{tabular}{|c|c|}
    \hline
      Facial regions   &  Predicted AUs\\
      \hline
      upper   &  AU1,AU2,AU4,AU7 \\
      \hline
      middle  &  AU6,AU9 \\ 
      \hline
      lower  & \makecell{AU9,AU10,AU12,AU14,AU15\\AU17,AU23,AU24,AU25,AU26} \\
      \hline
    \end{tabular}
    \caption{AU-region mapping rule}
    \label{tab:rules}
\end{table}
% \begin{figure}
%     \centering
%     \includegraphics[width=0.9\linewidth]{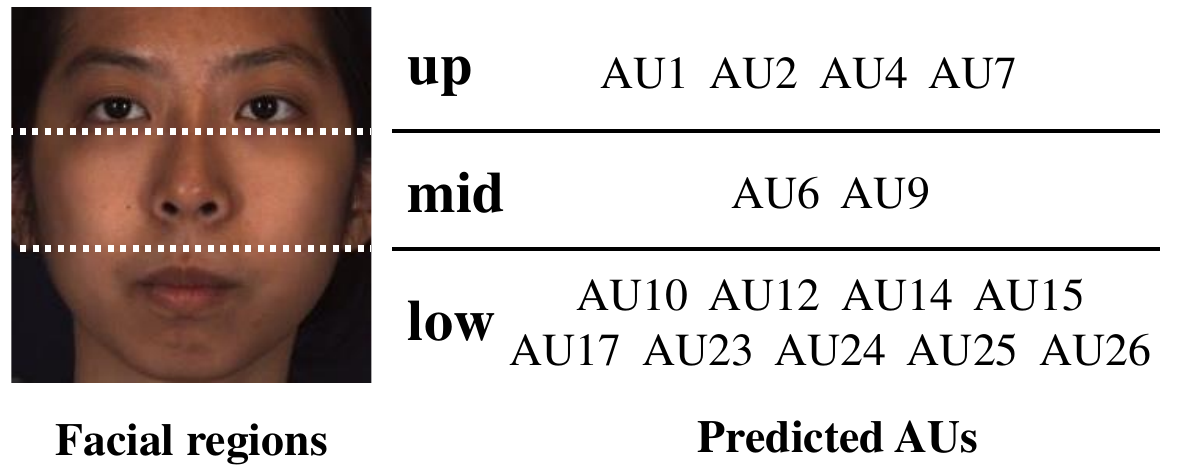}
%     \caption{Enter Caption}
%     \label{fig:enter-label}
% \end{figure}

\section{Dataset label distribution}

We provide the AU occurrence label distribution of the employed BP4D and DISFA datasets in Figure \ref{fig:BP4D_distribution} and Figure \ref{fig:DISFA_distribution}. It is clear that for the majority of target AUs, the number of inactivated frames are much more than the frames where they are occurred. Meanwhile, data imbalance also exists between each AU class.

\definecolor{mycolor1}{HTML}{f4b183} 
\definecolor{mycolor2}{HTML}{9dc3e6}
\begin{figure*}
    \centering
\scalebox{0.95}{
\begin{tikzpicture}
    \begin{axis}[
        ybar,
        x = 1.4cm,
        ymajorgrids=true,
        symbolic x coords={AU1,AU2,AU4,AU6,AU7,AU10,AU12,AU14,AU15,AU17,AU23,AU24},
        xtick=data,
        ylabel=Number of Samples,
        ylabel style={font=\small, yshift=-10pt},
        legend style={at={(0.5,1.0)}, font=\small, anchor=north, legend columns=-1},
        axis y line=left,
        axis x line=bottom,
        nodes near coords,
        nodes near coords style={
            font=\scriptsize,
            /pgf/number format/sci,
            /pgf/number format/precision=1,
            color=black,
            xshift=4pt,
            yshift=0pt,
        },
        tick label style={font=\small},  % 调整坐标轴刻度的字体大小
        ymin=0,
        enlarge x limits=0.05 
        ]
		\addplot+[fill=mycolor1, draw=black] coordinates {(AU1, 31042) (AU2, 25110) (AU4, 29755) (AU6, 67676) (AU7,80616) (AU10,87270) (AU12,82530) (AU14, 68375) (AU15, 24869) (AU17,50406) (AU23,24288) (AU24,22229)};
		\addplot+[fill=mycolor2, draw=black] coordinates {(AU1, 115805) (AU2, 121737) (AU4, 117092) (AU6, 79171) (AU7,66231) (AU10,59577) (AU12,64317) (AU14,78472) (AU15, 121978) (AU17,96441) (AU23,122559) (AU24,124618)}; 
		\legend{activate,inactivate}; 
	\end{axis} 
\end{tikzpicture}
}
\vspace{-0.1cm}
\caption{Label distribution on BP4D}
\label{fig:BP4D_distribution}
\end{figure*}

\vspace{+0.2cm}

\begin{figure*}
    \centering
\scalebox{0.95}{
\begin{tikzpicture}
    \begin{axis}[
        ybar,
        x = 1.8cm,
        ymajorgrids=true,
        symbolic x coords={AU1,AU2,AU4,AU6,AU9,AU12,AU25,AU26},
        xtick=data,
        ylabel=Number of Samples,
        ylabel style={font=\small, yshift=-10pt},
        legend style={at={(0.82,1.0)}, font=\small, anchor=north, legend columns=1},
        axis y line=left,
        axis x line=bottom,
        nodes near coords,
        nodes near coords style={
            font=\scriptsize,
            /pgf/number format/sci,
            /pgf/number format/precision=1,
            color=black,
            xshift=4pt,
            yshift=0pt,
        },
        enlarge x limits=0.1,
        ymin=0,
        ymax=135000,
        tick label style={font=\small},  % 调整坐标轴刻度的字体大小
        ] 
        \addplot+[fill=mycolor1, draw=black] coordinates {(AU1, 6506) (AU2, 5644) (AU4, 19933) (AU6, 10327) (AU9,5473) (AU12,16851) (AU25,36247) (AU26,11533)}; 
        \addplot+[fill=mycolor2, draw=black] coordinates {(AU1, 124308) (AU2, 125170) (AU4, 110881) (AU6, 120487) (AU9,125341) (AU12,113963) (AU25,94567) (AU26,119281)}; 
        \legend{activate,inactivate}; 
    \end{axis} 
\end{tikzpicture} 
}

\caption{Label distribution on DISFA}
\label{fig:DISFA_distribution}
\vspace{-0.1cm}
\end{figure*}

\section{Training details}
% We follow previous approaches \cite{Zhang_2018_CVPR,shao2021jaa} to apply MTCNN \cite{zhang2016joint} to crop and align a $224 \times 224$ face region from each frame, and conduct subject-independent three-folds cross-validation for each dataset, where the reported results are achieved by averaging the validation results of three folds. We pad $k$ frames that same to the first frame / last frame at the beginning / end of each face video to ensure all frames can be processed by our model. AdamW \cite{loshchilov2018decoupled} optimizer with $\beta_1 = 0.9$, $\beta_2 = 0.999$ is employed for training and the $\lambda$ in Eq. \ref{loss_weight} is set to 0.01. A cosine decay learning rate scheduler is utilized, with an initial value of $10e^{-4}$. Both backbones are pre-trained on ImageNet \cite{deng2009imagenet}. All our experiments are conducted using NVIDIA A100 GPUs based on the open-source PyTorch library. More detailed model, training/validation, and dataset settings are provided in the Supplementary Material.

During the training, we only randomly select one image sequence of $T$ frames from each video at each epoch, i.e., not all training examples are used for training at each training epoch. Thus, we train our model for with maximum 200 epochs. In the testing phase, all videos are split into image segments of length $T$. The number of input frame $T$, the number of adjacent frames $k$ and the mini-batch size are set to 16, 5 and 8, respectively, for all our experiments. The detailed hyper-parameter settings of two backbone (ResNet and Swin-Transformer)-based best systems on BP4D and DISFA datasets are provided in Table \ref{tab:hyper-parameter}. \textbf{We used this hyper-parameter setting for training two backbone-based systems on both datasets}, suggesting that our approach is robust. In other words, individually and specifically tuning hyper-parameters for each system on each dataset may lead our approach to achieve even more promising performances.

\begin{table}[h!]
    \centering
    \begin{tabular}{cc}
    \toprule
     parameters    &  values\\
     \midrule
     Batch size    &   8   \\
     Learning rate &  0.0001 \\
     Training epochs        &    200  \\
     Validation interval & 25 \\
     Weight decay  &   0.0005 \\
     Crop size     &  $224\times 224$\\
     T             &16\\
     k             &5\\
     $\lambda $      &0.01\\
     $\beta_1$        &0.9\\
     $\beta_2$        &0.999 \\     \bottomrule
    \end{tabular}
    \caption{hyper-parameter settings}
    \label{tab:hyper-parameter}
    \vspace{-0.3cm}
\end{table}

% %%%%%%%%
%In the validation phase, videos are split into clips of length $L$, with 

%and the weight decay is set to $5e^{-4}$. The loss weight $\lambda$ in Eq. \ref{loss_weight} is set to 0.01. A cosine decay learning rate scheduler is utilized, with an initial value of $5e^{-4}$. Both backbones are pre-trained on ImageNet \cite{deng2009imagenet}. In the testing phase, test video are split into clips of length $L$, with padding using the last frame if needed. All our experiments are conducted using NVIDIA A100 GPUs based using the open-source PyTorch library.

% We train the model for with maximum 200 epochs, where in each epoch $L$ continuous frames are randomly sampled as input sequences from every videos in the training set, the number of frame $L$ and the mini-batch size are set to 16 and 8. we employ an AdamW \cite{} optimizer with $\beta_1 = 0.9$, $\beta_2 = 0.999$ and weight decay of $5e^{-4}$. The loss weight $\lambda$ in Eq. \ref{loss_weight} is set to 0.01. A cosine decay learning rate scheduler is utilized, with an initial value of $5e^{-4}$. Both backbones are pre-trained on ImageNet \cite{deng2009imagenet}. In the testing phase, test video are split into clips of length $L$, with padding using the last frame if needed. All our experiments are conducted using NVIDIA A100 GPUs based using the open-source PyTorch library.

\section{Parameter sensitivity analysis}

\textbf{Time-window length $k$:} Table \ref{tab:k} displays the parameter sensitive analysis results in terms of the `$k$' on the BP4D dataset. It can be observed that this parameter moderately impacts the performance, with the best F1 results of 66.6\% achieved at $k=5$. Importantly, our model can consistently and effectively capture AU recognition-related temporal cues under most time-window sizes, indicating that our approach is robust and effective. Nevertheless, an appropriate context window sizes allows the model to more effectively capture useful facial dynamics and spatio-temporal cues, while excessive or insufficient adjacent frames provide less meaningful facial dynamic cues. 
\begin{table}[ht]
    \vspace{-0.1cm}
    \setlength{\tabcolsep}{0.9mm}{
    \centering
    \begin{tabular}{c|cccccccc}
    \toprule
        $k$ & 1 & 2 & 3 & 4 & 5 & 6 & 7 & 8  \\
    \midrule  
        F1-score&65.8&65.7&66.2&65.9&66.6&66.5&65.8&65.9 \\
    \bottomrule
    \end{tabular}
   
    \caption{Sensitive analysis of $k$ in terms of average F1-scores (in \%) achieved on BP4D dataset.}
    \label{tab:k}
    }
    \vspace{-0.4cm}
\end{table}

\textbf{Loss weighting parameter $\lambda$:} Table \ref{tab:lambda} presents the F1-scores achieved by our approach on the BP4D dataset with different $\lambda$ values, which balances the importance between the main task loss and the auxiliary regional prediction loss during training. It can be seen that $\lambda$ significantly influences model performance. Even using very small $\lambda$ values (e.g., 0.0001 or 0.001) leads to improved performance compared to $\lambda=0$, with F1-scores increasing from 65.9 \% to 66.2\% and 66.3\% respectively. This indicates that a slight weighting on regional prediction task helps the model generalize better, where the optimal F1-score of 66.6\% is obtained at $\lambda=0.01$. However, when $\lambda$ value is too large (i.e., more than 0.05), our model performance starts to degrades. This implies excessive emphasis on the regional prediction over the main task is harmful for the model training.
\begin{table}[ht]
\setlength{\tabcolsep}{0.9mm}{
    \centering
    \begin{tabular}{c|cccccccc}
    \toprule
       $\lambda$& 0 & 0.0001 & 0.001 &0.01 & 0.05 &0.1&0.2&0.5 \\
    \midrule
          F1-score   & 65.9&66.2&66.3&66.6&66.0&65.6&65.3&64.8 \\
    \bottomrule
    \end{tabular}
    \caption{Sensitive analysis of $\lambda$ in terms of average F1-scores (in \%) achieved on BP4D dataset.}
    \label{tab:lambda}
    }
    \vspace{-0.3cm}
\end{table}

\section{Model complexity analysis}

Our model is very efficient as it has low FLOPs per frame, which makes our model very efficient for real applications. We compare our graph-based model with previous state-of-the-art ME-GraphAU model (based on their publicly available code) in Table \ref{tab:my_label}, where our approach has clearly lower FLOPs per frame compared to ME-GraphAU but better AU recognition performance. This is because that the characteristics that ours takes a video clip as input and predicts for all frames together. In summary, our model has a powerful architecture but is still lightweight for video facial analysis. By predicting all frames together, it reduces computations compared to models that process each frame individually.

\begin{table}[ht]
    \centering
    \begin{tabular}{c|c|c}
    \toprule
       Method  & Params  &FLOPs \\
    \midrule
       ME-GraphAU   & 93.3M    & 36.0G  \\
       MDHR(ResNet50)  & 91.09M   & 7.18G \\
       MDHR(Swin-base)  &  105.94M  & 15.99G   \\
    \bottomrule
    \end{tabular}
    \caption{Parameters and FLOPs of our model.}
    \vspace{-0.3cm}
    \label{tab:my_label}
\end{table}

\section{Statistical significance analysis}

We investigate the statistical significance differences between different variants of our approach by conducting paired t-tests on predictions achieved for the BP4D dataset, where the backbone is the ResNet50. As shown in Table \ref{tab:t-Tests}, the returned P values of all paired comparisons are lower than the confidence threshold of 0.05. This indicates that: (i) the proposed MFD and HSR brought significant improvements in terms of AU recognition; and (ii) MFD and HSR can encode crucial complementary AU-related cues, leading MDHR to significantly better than Backbone+MFD and Backbone+HSR systems.

\begin{table}[h]
    \centering
    \scalebox{0.9}{
    \begin{tabular}{c|c|c}
    \toprule
      Method &\makecell{Significant \\difference ?} &  P-value\\
     \midrule  
     Backbone+MFD vs Backbone & Yes & $7.75 \times 10^{-3}$ \\
     Backbone+HSR vs Backbone & Yes&$5.43 \times 10^{-3}$ \\
     MDHR vs Backbone & Yes  & $6.76 \times 10^{-6}$ \\
     MDHR vs Backbone+MFD & Yes & $8.26 \times 10^{-5}$ \\
     MDHR vs Backbone+HSR &  Yes & $1.53\times 10^{-2}$ \\     
    \bottomrule
    \end{tabular}
    }
    \caption{Statistical significance analysis results, where we set the confidence of 0.05.}
    \label{tab:t-Tests}
\end{table}
